# Supplementary material for: Fundamental Limits on Measuring the Rotational Constraint of Single Molecules using Fluorescence Microscopy
Source: arXiv:1811.09017 ancillary file (2019-04-19)
Supplement: Supplementary file 1 [file SI.pdf]

# Supplemental Information for "Fundamental Limits on Measuring the Rotational Constraint of Single Molecules using Fluorescence Microscopy"

Oumeng Zhang and Matthew D. Lew*

*Department of Electrical and Systems Engineering,*

*Washington University in St. Louis, Missouri 63130, USA*

## I. METHODS OF MEASURING DIPOLE ORIENTATION

### A. In-plane excitation polarization modulation

A linearly-polarized illumination beam was assumed to be modulated by an electro-optic modulator (EOM, Fig. S1(a)), which rotates its linear polarization vector to an arbitrary vector $\boldsymbol{E}_i = [E_{x,i}, E_{y,i}]$ in the sample plane. Since the captured emission intensity of a single molecule (SM) is proportional to the SM's absorption probability, the photons detected from the SM (at IIP, Fig. S1(a)) in each measurement are given by (Eq. (2)) [1]

$$g_i \propto \langle |\boldsymbol{E}_i \cdot \boldsymbol{\mu}|^2 \rangle \propto |E_{x,i}|^2 \langle \zeta_x^2 \rangle + |E_{y,i}|^2 \langle \zeta_y^2 \rangle + 2\mathcal{R}(E_{x,i}E_{y,i}) \langle \zeta_x \zeta_y \rangle \tag{S1}$$

The angle brackets $\langle \cdot \rangle$ denote the temporal average taken over one camera frame. Since rotational correlation times are typically much shorter than camera integration times, it can be viewed as an equivalent average over the full range orientations explored by a molecule. In cases of longer rotational correlation times, measurements of rotational constraint may complement long-term orientation tracking by revealing different rotational motions over different timescales, e.g., for a fluorophore embedded within a polymer [2].

We analyze the case of using 3 excitation polarizations, and the resulting images of an emitter are shown in Fig. S1(b). A $3 \times 3$ matrix (Fig. S2(a))

$$\boldsymbol{B}_{\text{ExMod}} = \begin{bmatrix} |E_{x,1}|^2 & |E_{y,1}|^2 & 2\mathcal{R}(E_{x,1}E_{y,1}) \\ |E_{x,2}|^2 & |E_{y,2}|^2 & 2\mathcal{R}(E_{x,2}E_{y,2}) \\ |E_{x,3}|^2 & |E_{y,3}|^2 & 2\mathcal{R}(E_{x,3}E_{y,3}) \end{bmatrix} \tag{S2}$$

* mdlew@wustl.edu

is calculated from Eq. (S1). For the simple symmetric excitation case modeled in the main text, i.e., $\boldsymbol{E}_1 \propto [1,0]^\dagger$, $\boldsymbol{E}_2 \propto [-1/2,-\sqrt{3}/2]^\dagger$, $\boldsymbol{E}_3 \propto [-1/2,\sqrt{3}/2]^\dagger$,

$$\boldsymbol{B}_{\text{ExMod}} = \begin{bmatrix} 2/3 & 0 & 0 \\ 1/6 & 1/2 & -\sqrt{3}/3 \\ 1/6 & 1/2 & \sqrt{3}/3 \end{bmatrix}. \tag{S3}$$

### B. Tri-spot point spread function (PSF)

A Tri-spot phase mask [2] that separates light in the back focal plane into three sub-regions creates Tri-spot images of SM emitters at the image plane (Fig. S1(c)) in both detection channels. Photons in each spot region are integrated for each of the basis images to form 6-element basis-image vectors. The basis-image matrix (Fig. S2(b))

$$\boldsymbol{B}_{\text{Tri-spot}} = \begin{bmatrix} 0.22 & 0 & 0.10 & -0.04 & -0.28 & 0.03 \\ 0.22 & 0 & 0.10 & -0.04 & 0.28 & -0.03 \\ 0.54 & 0.01 & 0.07 & 0.06 & 0 & 0 \\ 0 & 0.22 & 0.10 & 0.04 & -0.03 & 0.28 \\ 0 & 0.22 & 0.10 & 0.04 & 0.03 & -0.28 \\ 0.01 & 0.54 & 0.07 & -0.06 & 0 & 0 \end{bmatrix} \tag{S4}$$

is represented by a $6 \times 6$ invertible matrix with each column representing a basis-image vector (the response of the Tri-spot PSF to a particular orientational second moment). The top 3 rows of $\boldsymbol{B}_{\text{Tri-spot}}$ represent photons collected in the $x$-polarized channel, while the bottom 3 rows represent the $y$-polarized channel.

### C. Standard point spread function

The image formation of the standard PSF is modeled similarly to that of the Tri-spot PSF. A clear aperture is applied to the back focal plane (Fig. S1(d)). The difference in data analysis is that we perform pixel-wise shape matching [3] with a pixel size small enough to detect fine details of the PSF. We simulated the performance of this technique using a pixel size of 58.5 nm in object space. Due to the lack of energy contained in $\boldsymbol{B}_{xz}$ and $\boldsymbol{B}_{yz}$, the basis-image matrix $\boldsymbol{B}_{\text{standard}}$ is of size $N \times 4$ where $N = 9 \times 9 \times 2$ is the number of pixels that sample the PSF across two polarization channels (an equivalent of $526.5 \times 526.5$ nm$^2$ [3.5× FWHM of the standard PSF], Fig. S2(c)).

### D. Back focal plane imaging

In this method, we assume that only one molecule is excited within the sample, e.g., by using focused confocal illumination. A camera placed at the back focal plane (BFP) after separating $x$ and $y$ polarizations is then used to capture the image [4] (Fig. S1(e)). We assume the same total number of signal and background photons as the standard PSF to facilitate a fair comparison. The basis-image matrix $\boldsymbol{B}_{\text{BFP}}$ of this method is of size $N \times 6$ (Fig. S2(d)), where $N = \lfloor \pi 80^2 \rceil \times 2$ is the number of pixels that sample the BFP, where $\lfloor \cdot \rceil$ denotes the rounding operator.

### E. Photon statistics of the analysis

The accuracy and precision of an orientation measurement method depend on not only the basis-image matrix, but also the detected signal and background photons. To perform a fair comparison among all orientation measurement methods, the signal and background photons captured must be carefully chosen. The signal photons from a single-molecule emitter varies due to the orientation-dependent collection efficiency of the microscope, i.e., the fluorescence emitted from a dipole exhibiting strong $\bar{\mu}_z$ is less efficiently collected than that from a dipole exhibiting strong $\bar{\mu}_x$ or $\bar{\mu}_y$. For the Tri-spot, standard PSF and BFP imaging, this effect is encoded in the basis-image matrix, that is, the basis-image matrix is normalized so that $\mathbf{1}^\dagger \boldsymbol{B}_{xx,\text{Tri-spot}} = \mathbf{1}^\dagger \boldsymbol{B}_{xx,\text{standard}} = \mathbf{1}^\dagger \boldsymbol{B}_{xx,\text{BFP}} = 1$ and $\mathbf{1}^\dagger \boldsymbol{B}_{zz,\text{Tri-spot}} = \mathbf{1}^\dagger \boldsymbol{B}_{zz,\text{standard}} = \mathbf{1}^\dagger \boldsymbol{B}_{zz,\text{BFP}} < 1$. For the excitation modulation method, since the forward model is not sensitive to $\mu_z$ (Eq. (2)), the scalar $s$ is scaled so that the total number of detected photons is equal to that of the other methods.

One choice for normalizing the number of background photons between methods is to simply assume that the entries $b_i$ in the background vector $\boldsymbol{b}$ for all methods are uniform, e.g., the background per single measurement using excitation modulation and per spot using Tri-spot PSF in Fig. 1(c) are identical. However, this choice ignores the differences in integration time and imaging area captured by the different methods. In Fig. 3, we assume a uniform amount (20) of background photons per unit area per unit time, that is, the photons were separated into two polarization channels (10 photons per pixel in each channel) for Tri-spot and Standard PSFs, and into three frames (6.67 photons per pixel in each frame) for in-plane excitation modulation. For the BFP imaging method, the total background was set to be equal to that of the standard PSF in a $526.5 \times 526.5$ nm$^2$ region. The total number of background photons in this comparison follows: $\mathbf{1}^\dagger \boldsymbol{b}_{\text{ExMod}} = \mathbf{1}^\dagger \boldsymbol{b}_{\text{BFP}} = \mathbf{1}^\dagger \boldsymbol{b}_{\text{standard}} = \mathbf{1}^\dagger \boldsymbol{b}_{\text{ideal}} = \mathbf{1}^\dagger \boldsymbol{b}_{\text{Tri-spot}}/3$ due to the three-times larger size of the

Tri-spot PSF.

## II. ROTATIONAL CONSTRAINT ANALYSIS

### A. In-plane (2D) methods

In the paper, we discussed a simplified case where the molecules' average orientation lies within the $xz$ plane, i.e. $\bar{\mu}_y = \bar{\zeta}_y = 0$. Here, we include the derivation of the bias in estimating rotational constraint for a more generalized case. The image-formation equation using an in-plane technique is given by

$$\boldsymbol{g} = s\left(\boldsymbol{B}_{xx}\langle\hat{\zeta_x^2}\rangle + \boldsymbol{B}_{yy}(1 - \langle\hat{\zeta_x^2}\rangle) + \boldsymbol{B}_{xy}\langle\widehat{\zeta_x\zeta_y}\rangle\right) + \boldsymbol{b} \tag{S5}$$

The $2 \times 2$ in-plane second-moment matrix can be decomposed as

$$\boldsymbol{M}_{2\text{D}} = \sum_{i=1}^{2} \lambda_i \boldsymbol{\nu}_i \boldsymbol{\nu}_i^\dagger = (2\lambda_1 - 1)\boldsymbol{\nu}_1\boldsymbol{\nu}_1^\dagger + (2 - 2\lambda_1)\frac{\boldsymbol{\nu}_1\boldsymbol{\nu}_1^\dagger + \boldsymbol{\nu}_2\boldsymbol{\nu}_2^\dagger}{2} = \gamma_{2\text{D}}\boldsymbol{\nu}_1\boldsymbol{\nu}_1^\dagger + (1 - \gamma_{2\text{D}})\frac{\boldsymbol{I}}{2} \tag{S6}$$

where $\gamma_{2\text{D}} = 2\lambda_1 - 1 = \sqrt{(2\langle\zeta_x^2\rangle - 1)^2 + (2\langle\zeta_x\zeta_y\rangle)^2}$ is the rotational constraint. The precision of $\langle\hat{\zeta_x^2}\rangle$ and $\langle\hat{\zeta_y^2}\rangle$ can be calculated by inverting the Fisher information matrix $\boldsymbol{\mathcal{I}}$ such that

$$\boldsymbol{\mathcal{I}} = \sum_i \frac{1}{g_i}\begin{bmatrix} \left(\frac{\partial g_i}{\partial\langle\zeta_x^2\rangle}\right)^2 & \frac{\partial g_i}{\partial\langle\zeta_x^2\rangle}\frac{\partial g_i}{\partial\langle\zeta_x\zeta_y\rangle} \\ \frac{\partial g_i}{\partial\langle\zeta_x^2\rangle}\frac{\partial g_i}{\partial\langle\zeta_x\zeta_y\rangle} & \left(\frac{\partial g_i}{\partial\langle\zeta_x\zeta_y\rangle}\right)^2 \end{bmatrix} = \sum_i \frac{s^2}{g_i}\begin{bmatrix} (B_{xx,i} - B_{yy,i})^2 & (B_{xx,i} - B_{yy,i})B_{xy,i} \\ (B_{xx,i} - B_{yy,i})B_{xy,i} & B_{xy,i}^2 \end{bmatrix},$$

$$\sigma_{xx} = \sigma^{\text{CRLB}}_{\langle\hat{\zeta_x^2}\rangle} = \sqrt{(\boldsymbol{\mathcal{I}}^{-1})_{11}}, \quad \sigma_{xy} = \sigma^{\text{CRLB}}_{\langle\widehat{\zeta_x\zeta_y}\rangle} = \sqrt{(\boldsymbol{\mathcal{I}}^{-1})_{22}} \tag{S7}$$

Further, if the off-diagonal terms in the Fisher information matrix are close to zero, i.e., the sensitivity of this method to measuring $\langle\hat{\zeta_x^2}\rangle$ is independent of its sensitivity to $\langle\widehat{\zeta_x\zeta_y}\rangle$ (this assumption holds for molecules under low constraint where the bias is most significant, e.g., $\mathcal{I}_{12}$ is less than 10% of $\mathcal{I}_{11}$ and $\mathcal{I}_{22}$ for a molecule with any average orientation and a rotational constraint of $\gamma_{2\text{D}} = 0.2$), the probability density function of $\hat{\gamma}_{2\text{D}}$ can be approximately computed as

$$p(\hat{\gamma}_{2\text{D}}) = 2\hat{\gamma}_{2\text{D}}\left(f_{(2\langle\zeta_x^2\rangle - 1), 2\sigma_{xx}} * f_{(2\langle\zeta_x\zeta_y\rangle), 2\sigma_{xy}}\right)\left(\hat{\gamma}_{2\text{D}}^2\right) \tag{S8}$$

where

$$f_{\mu,\sigma}(x) = \frac{1}{2\sigma^2}\exp\left(-\frac{x + \mu^2}{2\sigma^2}\right)\left(\frac{x}{\mu^2}\right)^{-1/4} I_{-1/2}\left(\frac{\mu\sqrt{x}}{\sigma^2}\right) \tag{S9}$$

is a scaled non-central chi-squared PDF. The operator $*$ represents convolution, and $I_\alpha(\cdot)$ is the modified Bessel function of the first kind.

For the simplified symmetric excitation case, the elements in the Fisher information matrix of a molecule with average orientation $\boldsymbol{\zeta} = [1, 0]^\dagger$ are $\boldsymbol{\mathcal{I}}_{11} = \boldsymbol{\mathcal{I}}_{22} = 1/\sigma^2$, $\boldsymbol{\mathcal{I}}_{12} = \boldsymbol{\mathcal{I}}_{21} = 0$. The rotational

constraint measurements $\hat{\gamma}_{2\text{D}}$ follow a non-central chi distribution with 2 degrees of freedom in Eq. (4). We verified that the computed PDF matches the estimates from a basis-inversion estimator using simulated images with Poisson noise (Fig. S4), i.e., we find the orientational second moments by inverting the basis-matrix

$$\hat{s}\left[\langle\hat{\zeta_x^2}\rangle, \langle\hat{\zeta_y^2}\rangle, \langle\hat{\zeta_x\zeta_y}\rangle\right]^\dagger = \boldsymbol{B}_{\text{ExMod}}^{-1}\boldsymbol{g} \tag{S10}$$

and estimate $\hat{\gamma}_{2\text{D}}$ using eigendecomposition (Eq. (S6), Fig. S3(a-d)). This estimator does not set any constraint on the range of the estimated second-order moments, i.e., even though $\langle\zeta_x^2\rangle \in [0,1]$, the estimated value $\langle\hat{\zeta_x^2}\rangle$ is allowed to be negative or greater than 1. The estimated second moments are then mapped to a rotational constraint $\hat{\gamma}$ that is not necessarily within [0,1], similar to the results shown in [1]. Therefore, we model the estimated second moments as unbiased Gaussian variables since we avoid adding artificial bias from a nonnegativity assumption.

For an isotropic emitter under uniform background $\boldsymbol{b}$, the captured images are given by $g_i = (s + \boldsymbol{1}^\dagger\boldsymbol{b})/3$. The CRLBs in estimating the second moments are thus $\sigma_{xx} = \sigma_{xy} = \sqrt{(s+\boldsymbol{1}^\dagger\boldsymbol{b})/2}/s$. Therefore, the expected estimates of in-plane rotational constraint are given by Eq. (5).

### B. Eigendecomposition of the 3D orientational second-moment matrix

The precision to which the second moments can be estimated is calculated in a similar manner as Section II A by inverting the Fisher information matrix

$$\boldsymbol{\mathcal{I}} = \sum_i \frac{s^2}{g_i}\left[B_{xx,i}, B_{yy,i}, B_{zz,i}, B_{xy,i}, B_{xz,i}B_{yz,i}\right]^\dagger \left[B_{xx,i}, B_{yy,i}, B_{zz,i}, B_{xy,i}, B_{xz,i}B_{yz,i}\right] \tag{S11}$$

For isotropic emitters imaged with the ideal basis-image matrix $\boldsymbol{B}_{\text{ideal}}$ (Fig. S2(e)), the captured images are given by $g_i = (s + \boldsymbol{1}^\dagger\boldsymbol{b})/6$. The off-diagonal elements in $\boldsymbol{\mathcal{I}}$ are zero, and the diagonal elements are uniform. The CRLBs for estimating the second moments are $\sigma_{\langle\mu_i\mu_j\rangle}^{\text{CRLB}} = \sqrt{(s+\boldsymbol{1}^\dagger\boldsymbol{b})/3}/s$.

Similarly, the assembled $3\times3$ 3D second-moment matrix can be represented using its eigenvalues $\lambda_i$ and eigenvectors $\boldsymbol{\nu}_i$

$$\begin{aligned}\boldsymbol{M}_{3\text{D}} = \sum_{i=1}^{3}\lambda_i\boldsymbol{\nu}_i\boldsymbol{\nu}_i^\dagger &= \left(\frac{3\lambda_1-1}{2}+\frac{1-\lambda_1}{2}\right)\boldsymbol{\nu}_1\boldsymbol{\nu}_1^\dagger + \sum_{j=2}^{3}\left(\frac{1-\lambda_1}{2}+(-1)^j\frac{\lambda_2-\lambda_3}{2}\right)\boldsymbol{\nu}_j\boldsymbol{\nu}_j^\dagger \\ &= \frac{3\lambda_1-1}{2}\boldsymbol{\nu}_1\boldsymbol{\nu}_1^\dagger + \frac{3-3\lambda_1}{2}\frac{\boldsymbol{I}}{3} + \frac{\lambda_2-\lambda_3}{2}(\boldsymbol{\nu}_2\boldsymbol{\nu}_2^\dagger - \boldsymbol{\nu}_3\boldsymbol{\nu}_3^\dagger)\end{aligned} \tag{S12}$$

where the rotational constraint $\gamma_{3\text{D}} = (3\lambda_1 - 1)/2$. We define a maximum likelihood estimator (MLE) for measuring rotational constraint that minimizes the log-likelihood

$$\Lambda(\hat{\boldsymbol{\mu}}, \hat{\gamma}_{3\text{D}}, \hat{s}, \boldsymbol{g}, \boldsymbol{b}) = \Sigma_{i=1}^{6}\left(g_i \ln(\hat{g}_i) - \hat{g}_i\right) \tag{S13}$$

where

$$\hat{g}_i = \hat{s}\boldsymbol{B}_{\text{Tri-spot}}\hat{\boldsymbol{m}}_{\mu\gamma} \tag{S14}$$

and $\hat{\boldsymbol{m}}_{\mu\gamma}$ represents the second-moment vector as a function of average orientation $\hat{\bar{\boldsymbol{\mu}}}$ and rotational constraint $\hat{\gamma}_{\text{3D}}$ [2]. Comparing the eigendecomposition using Eq. (S12) to the MLE (Eq. (S13)) run on simulated images, we find that the resulting measurement distributions of rotational constraint $\hat{\gamma}_{3D}$ match very well (Fig. S5). The observed bias and standard deviation of the estimates are within 9% and 6% for isotropic emitters, respectively.

### C. Measuring rotational constraint from a subset of orientational second moments

We assemble a truncated three-dimensional second-moment matrix, similar to that measured by in-plane excitation modulation, as

$$\boldsymbol{M}_{\text{3D,t}} = \begin{bmatrix} \langle\mu_x^2\rangle & \langle\mu_x\mu_y\rangle \\ \langle\mu_x\mu_y\rangle & \langle\mu_y^2\rangle \end{bmatrix} \tag{S15}$$

The 3D rotational constraint of a dipole emitter is computed as a function of the eigenvalues of $\boldsymbol{M}_{\text{3D,t}}$, given by

$$\lambda_1 = \gamma_{\text{3D}}(\bar{\mu}_x^2 + \bar{\mu}_y^2) + \frac{1-\gamma_{\text{3D}}}{3}, \quad \lambda_2 = \frac{1-\gamma_{\text{3D}}}{3} \tag{S16}$$

The in-plane rotational constraint can be computed as $\gamma_{\text{2D}} = (\lambda_1 - \lambda_2)/(\lambda_1 + \lambda_2)$ (Eq. (8)) [1]. For the standard PSF, we compute $\hat{\gamma}_{\text{3D}}$ from the measured second moments using the relations

$$\hat{\gamma}_{\text{3D}}\hat{\bar{\mu}}_x^2 + \frac{1-\hat{\gamma}_{\text{3D}}}{3} = \widehat{\langle\mu_x^2\rangle} \tag{S17}$$

$$\hat{\gamma}_{\text{3D}}\hat{\bar{\mu}}_y^2 + \frac{1-\hat{\gamma}_{\text{3D}}}{3} = \widehat{\langle\mu_y^2\rangle} \tag{S18}$$

$$\hat{\gamma}_{\text{3D}}\hat{\bar{\mu}}_x\hat{\bar{\mu}}_y = \widehat{\langle\mu_x\mu_y\rangle} \tag{S19}$$

as

$$\hat{\gamma}_{\text{3D}} = 1 - \frac{3}{2}\left(\widehat{\langle\mu_x^2\rangle} + \widehat{\langle\mu_y^2\rangle} - \sqrt{\left(\widehat{\langle\mu_x^2\rangle} - \widehat{\langle\mu_y^2\rangle}\right)^2 + \left(2\widehat{\langle\mu_x\mu_y\rangle}\right)^2}\right). \tag{S20}$$

We implemented Monte-Carlo simulations to find biases, standard deviations, and probability densities for measurements of rotational constraint (Figs. 3, S7).

To better explain the procedure to find the measurement distribution of 3D rotational constraint using the symmetric in-plane excitation modulation, we rewrite Eq. (8) and Eq. (9) as

$$\gamma_{\mathrm{2D}} = h(\gamma_{\mathrm{3D}}, \bar{\mu}_z) \tag{S21}$$

$$\gamma_{\mathrm{3D}} = h^{-1}(\gamma_{\mathrm{2D}}, \bar{\mu}_z) \tag{S22}$$

$$\frac{\partial \gamma_{\mathrm{2D}}}{\partial \gamma_{\mathrm{3D}}} = h'(\gamma_{\mathrm{3D}}, \bar{\mu}_z) \tag{S23}$$

$$\frac{\partial \gamma_{\mathrm{3D}}}{\partial \gamma_{\mathrm{2D}}} = (h^{-1})'(\gamma_{\mathrm{2D}}, \bar{\mu}_z) \tag{S24}$$

where $h$ represents the 2D rotational constraint $\gamma_{\mathrm{2D}}$ in terms of the 3D rotational constraint $\gamma_{\mathrm{3D}}$ and average out-of-plane orientation $\bar{\mu}_z$. The distribution of $\hat{\gamma}_{\mathrm{3D}}$ can therefore be computed using

$$p(\hat{\gamma}_{\mathrm{3D}}) = h'(\hat{\gamma}_{\mathrm{3D}}, \bar{\mu}_z) \frac{h(\hat{\gamma}_{\mathrm{3D}}, \bar{\mu}_z)}{4\sigma^2} \exp\left(-\frac{h^2(\hat{\gamma}_{\mathrm{3D}}, \bar{\mu}_z) + h^2(\gamma_{\mathrm{3D}}, \bar{\mu}_z)}{8\sigma^2}\right) I_0\left(\frac{h(\hat{\gamma}_{\mathrm{3D}}, \bar{\mu}_z) h(\gamma_{\mathrm{3D}}, \bar{\mu}_z)}{4\sigma^2}\right) \tag{S25}$$

similarly to Eq. (4), where $\gamma_{\mathrm{3D}}$ is the true rotational constraint. The measurement average and standard deviation are approximated as

$$\bar{\hat{\gamma}}_{\mathrm{3D}} = h^{-1}(\bar{\hat{\gamma}}_{\mathrm{2D}}, \bar{\mu}_z) \bar{\hat{\gamma}}_{\mathrm{2D}} \tag{S26}$$

$$\mathrm{std}(\hat{\gamma}_{\mathrm{3D}}) = (h^{-1})'(\bar{\hat{\gamma}}_{\mathrm{2D}}, \bar{\mu}_z) \mathrm{std}(\hat{\gamma}_{\mathrm{2D}}) \tag{S27}$$

The full measurement distribution, as well as the predicted bias and standard deviation, match the output of the aforementioned basis-inversion estimator (Section II A) on simulated images with noise (Fig. S6) after converting the results to 3D space using Eq. (S22) (Fig. S3).

### D. Ideal basis-image matrix under a loose intensity constraint

Our goal is to construct a $6 \times 6$ basis image matrix $\boldsymbol{B}_{\mathrm{ideal}}$ to achieve the best-possible precision in estimating second moments using an information-theoretic approach. First, we evaluate the precision of estimating a subset of second moments $\langle \mu_x^2 \rangle$, $\langle \mu_y^2 \rangle$ and $\langle \mu_z^2 \rangle$ without considering $\boldsymbol{B}_{xy}$, $\boldsymbol{B}_{xz}$ and $\boldsymbol{B}_{yz}$. The sum of the basis images corresponding to these second moments must satisfy $\mathbf{1}^\dagger \boldsymbol{B}_{xx}, \mathbf{1}^\dagger \boldsymbol{B}_{yy}, \mathbf{1}^\dagger \boldsymbol{B}_{zz} \in [0, 1]$. These basis images represent the image corresponding to $x$-, $y$- and $z$-oriented molecules. Therefore, all pixel values $B_{xx,i}$, $B_{yy,i}$, and $B_{zz,i}$ must be nonnegative, where $i$ represents the pixel index. The Fisher information matrix of estimating this subset of second moments is

$$\boldsymbol{\mathcal{I}}_{\mathrm{sub}} = \sum_{i=1}^{6} \frac{s^2}{g_i} \begin{bmatrix} B_{xx,i}^2 & B_{xx,i}B_{yy,i} & B_{xx,i}B_{zz,i} \\ B_{xx,i}B_{yy,i} & B_{yy,i}^2 & B_{yy,i}B_{zz,i} \\ B_{xx,i}B_{zz,i} & B_{yy,i}B_{zz,i} & B_{zz,i}^2 \end{bmatrix}, \tag{S28}$$

where $g_i$ is the intensity of the $i$th pixel in the captured image. The sum of the CRLBs of these second moments is bounded by

$$\left(\sigma_{\langle\hat{\mu_x^2}\rangle}^{\text{CRLB}}\right)^2 + \left(\sigma_{\langle\hat{\mu_y^2}\rangle}^{\text{CRLB}}\right)^2 + \left(\sigma_{\langle\hat{\mu_z^2}\rangle}^{\text{CRLB}}\right)^2 = \sum \text{eig}(\boldsymbol{\mathcal{I}}_{\text{sub}}^{-1}) \geq \frac{9}{\sum \text{eig}(\boldsymbol{\mathcal{I}}_{\text{sub}})} = \frac{9}{\text{tr}(\boldsymbol{\mathcal{I}}_{\text{sub}})}. \tag{S29}$$

The equality is satisfied when the eigenvalues of $\boldsymbol{\mathcal{I}}$ are uniform.

For isotropic emitters under zero background, the trace of $\boldsymbol{\mathcal{I}}$ is bounded by

$$\begin{aligned}
\text{tr}(\boldsymbol{\mathcal{I}}_{\text{sub}}) &= \sum_i \frac{(sB_{xx,i})^2}{g_i} + \sum_i \frac{(sB_{yy,i})^2}{g_i} + \sum_i \frac{(sB_{zz,i})^2}{g_i} \\
&\leq \sum_i \frac{(sB_{xx,i})^2}{sB_{xx,i}/3} + \sum_i \frac{(sB_{yy,i})^2}{sB_{yy,i}/3} + \sum_i \frac{(sB_{zz,i})^2}{sB_{zz,i}/3} \\
&= 3s\left(\sum_i B_{xx,i} + \sum_i B_{yy,i} + \sum_i B_{zz,i}\right) \leq 9s.
\end{aligned} \tag{S30}$$

To achieve this bound, only one of $B_{xx,i}$, $B_{yy,i}$ and $B_{zz,i}$ can be non-zero for any pixel $i$, and the energy of each basis image should be maximized, i.e., $\mathbf{1}^\dagger\boldsymbol{B}_{xx} = \mathbf{1}^\dagger\boldsymbol{B}_{yy} = \mathbf{1}^\dagger\boldsymbol{B}_{zz} = 1$. A $6 \times 3$ sub-basis-image matrix that satisfies these conditions is

$$[\boldsymbol{B}_{xx}, \boldsymbol{B}_{yy}, \boldsymbol{B}_{zz}] = \begin{bmatrix} 1-\epsilon_x & 0 & 0 \\ 0 & 1-\epsilon_y & 0 \\ 0 & 0 & 1-\epsilon_z \\ \epsilon_x & 0 & 0 \\ 0 & \epsilon_y & 0 \\ 0 & 0 & \epsilon_z \end{bmatrix}, \tag{S31}$$

where $\epsilon_x, \epsilon_y, \epsilon_z \in [0, 1/2]$ ($\epsilon_x, \epsilon_y, \epsilon_z \in [1/2, 1]$ represents the same matrix with swapped rows). This sub-basis-image matrix satisfies the equalities in Eqs. (S29,S30) simultaneously.

Now we include the basis images $\boldsymbol{B}_{xy}$, $\boldsymbol{B}_{xz}$ and $\boldsymbol{B}_{yz}$. These basis images correspond to the second moments $\langle\mu_x\mu_y\rangle$, $\langle\mu_x\mu_z\rangle$ and $\langle\mu_y\mu_z\rangle$. Since we prefer an imaging system with uniform photon collection efficiency, the total intensity collected from molecules with any orientation, regardless of being freely rotating or fixed, must be identical, i.e., $\mathbf{1}^\dagger\boldsymbol{B}_{xx} = \mathbf{1}^\dagger\boldsymbol{B}_{yy} = \mathbf{1}^\dagger\boldsymbol{B}_{zz} = \mathbf{1}^\dagger(\boldsymbol{B}_{\text{ideal}}\boldsymbol{m}) = 1$ where $\boldsymbol{m}$ is the second-moment vector. That is, the total energy within each basis image, corresponding to mixed second moments, must satisfy $\mathbf{1}^\dagger\boldsymbol{B}_{xy} = \mathbf{1}^\dagger\boldsymbol{B}_{xz} = \mathbf{1}^\dagger\boldsymbol{B}_{yz} = 0$. We next introduce a loose bound on the pixel values of $B_{xy,i}$, $B_{xz,i}$ and $B_{xz,i}$ similar to the other basis images. We consider molecules with uniform strength in all second order moments, i.e., $\langle\mu_x^2\rangle = \langle\mu_y^2\rangle = \langle\mu_z^2\rangle = |\langle\mu_x\mu_y\rangle| = |\langle\mu_x\mu_z\rangle| = |\langle\mu_y\mu_z\rangle| = 1/3$. The pixel values of the final image must be

nonnegative, i.e.,

$$|B_{xy,i}| + |B_{xz,i}| + |B_{yz,i}| \leq B_{xx,i} + B_{yy,i} + B_{zz,i}. \tag{S32}$$

Similarly, we want the absolute energy contribution from each second moment to be large and mutually orthogonal. We therefore write a $6 \times 6$ basis image matrix

$$[\boldsymbol{B}_{xx}, \boldsymbol{B}_{yy}, \boldsymbol{B}_{zz}, \boldsymbol{B}_{xy}, \boldsymbol{B}_{xz}, \boldsymbol{B}_{yz}] = \begin{bmatrix} 1-\epsilon_x & 0 & 0 & \epsilon_x & 0 & 0 \\ 0 & 1-\epsilon_y & 0 & 0 & \epsilon_y & 0 \\ 0 & 0 & 1-\epsilon_z & 0 & 0 & \epsilon_z \\ \epsilon_x & 0 & 0 & -\epsilon_x & 0 & 0 \\ 0 & \epsilon_y & 0 & 0 & -\epsilon_y & 0 \\ 0 & 0 & \epsilon_z & 0 & 0 & -\epsilon_z \end{bmatrix}. \tag{S33}$$

The $6 \times 6$ full Fisher information matrix for estimating all second moments corresponding to this basis-image matrix is given by

$$\boldsymbol{\mathcal{I}} = 3s \text{ diag}\left(1, 1, 1, \frac{\epsilon_x}{1-\epsilon_x}, \frac{\epsilon_y}{1-\epsilon_y}, \frac{\epsilon_z}{1-\epsilon_z}\right). \tag{S34}$$

The trace $\text{tr}(\boldsymbol{\mathcal{I}})$ is maximized when $\epsilon_x = \epsilon_y = \epsilon_z = 1/2$, i.e., the sum of the CRLBs of estimating all the second moments is minimized when

$$[\boldsymbol{B}_{xx}, \boldsymbol{B}_{yy}, \boldsymbol{B}_{zz}, \boldsymbol{B}_{xy}, \boldsymbol{B}_{xz}, \boldsymbol{B}_{yz}] = \frac{1}{2}\begin{bmatrix} \boldsymbol{I}_3 & \boldsymbol{I}_3 \\ \boldsymbol{I}_3 & -\boldsymbol{I}_3 \end{bmatrix}. \tag{S35}$$

One note is that this ideal basis-image matrix and the fundamental limit in Eq. (11) are derived by maximizing the Fisher information under a loose physical constraint. Non-negative intensity of the image is only guaranteed for molecules with orientations of $\boldsymbol{\mu} \in \{[\pm 1, 0, 0]^\dagger, [0, \pm 1, 0]^\dagger, [0, 0, \pm 1]^\dagger, [\pm\sqrt{(1/3)}, \pm\sqrt{(1/3)}, \pm\sqrt{(1/3)}]^\dagger\}$. For any physically realizable imaging system, the intensity of the $i$th pixel in the image is given by

$$g_i = \frac{1}{2} s \boldsymbol{\mu}^T \begin{bmatrix} 2B_{xx,i} & B_{xy,i} & B_{xz,i} \\ B_{xy,i} & 2B_{yy,i} & B_{xz,i} \\ B_{xz,i} & B_{yz,i} & 2B_{zz,i} \end{bmatrix} \boldsymbol{\mu} \geq 0. \tag{S36}$$

Therefore, each pixel of the basis image matrix must be positive semidefinite, that is

$$\begin{bmatrix} 2B_{xx,i} & B_{xy,i} & B_{xz,i} \\ B_{xy,i} & 2B_{yy,i} & B_{xz,i} \\ B_{xz,i} & B_{yz,i} & 2B_{zz,i} \end{bmatrix} \succeq 0. \tag{S37}$$

Under this constraint, the equality in Eq. (S30) implies that $B_{xy,i} = B_{xz,i} = B_{yz,i} = 0$ for all $i$. Therefore, in order to have sensitivity towards the second moments $\langle \mu_x \mu_y \rangle$, $\langle \mu_x \mu_z \rangle$ and $\langle \mu_y \mu_z \rangle$, the equality in Eq. (S30) cannot be satisfied. This result implies that any realistic imaging system will have worse precision in estimating the second moments compared to $\boldsymbol{B}_{\text{ideal}}$, i.e., its bias in measuring rotational constraint must be larger than what we derived in Eq. (11).

### E. Other measures of rotational diffusion

Quantities other than rotational constraint, e.g., linear dichroism (LD) and anisotropy factor $r$ [5], are also used for quantifying the wobble of fluorescent molecules. To analyze their relation to rotational constraint $\gamma$, we assemble a similar basis-image matrix using only $x$- and $y$- polarized emission separation:

$$\boldsymbol{B}_{\text{LD}} = \begin{bmatrix} B_{xx,x} & B_{yy,x} & B_{zz,x} \\ B_{xx,y} & B_{yy,y} & B_{zz,y} \end{bmatrix} = \frac{1}{2} \begin{bmatrix} 1+\Delta B & 1-\Delta B & B_z \\ 1-\Delta B & 1+\Delta B & B_z \end{bmatrix}, \tag{S38}$$

where $B_{ii,j}$ represents the integrated intensity in the $j$-channel emitted from the molecule's second moment component $\langle \mu_i^2 \rangle$. The quantity $\Delta B$, which is a property of the imaging system, represents the difference in $x$- and $y$-polarized emission intensity from an $x$-orientated molecule. It is usually close to one when the sample's refractive index matches the imaging medium (0.98 using an $NA = 1.4$ objective lens and $n = 1.5$ imaging medium). $B_z$ represents the captured intensity emitted from a $z-$orientated molecule, normalized by that of an $x$-orientated molecule.

The measured LD of a molecule can be computed based on its 3D rotational constraint $\gamma_{3\text{D}}$ and the average orientation $\bar{\boldsymbol{\mu}} = [\bar{\mu}_x, \bar{\mu}_y, \bar{\mu}_z]^\dagger$, such that

$$LD = \frac{I_x - I_y}{I_x + I_y} = \frac{3\gamma_{3\text{D}}(\bar{\mu}_x^2 - \bar{\mu}_y^2)\Delta B}{4 - B_z + (3\bar{\mu}_z^2 - 1)(1 - B_z)\gamma_{3\text{D}}}. \tag{S39}$$

An equivalent anisotropy factor [5] is given by

$$r = \frac{2\gamma_{3\text{D}}(\bar{\mu}_x^2 - \bar{\mu}_y^2)\Delta B}{4 - B_z + ((3\bar{\mu}_z^2 - 1)(1 - B_z) - (\bar{\mu}_x^2 - \bar{\mu}_y^2)\Delta B)\gamma_{3\text{D}}} \tag{S40}$$

For example, if a molecule exhibits an average orientation of $\bar{\boldsymbol{\mu}} = [\sqrt{2/3}, 0, \sqrt{1/3}]^\dagger$, its LD scales linearly with its 3D rotational constraint, that is

$$LD = \frac{2\gamma_{3\text{D}}\Delta B}{4 - B_z}. \tag{S41}$$

Its ansiotropy factor $r$ monotonically increases with $\gamma_{3\text{D}}$ as well,

$$r = \frac{2}{(12 - 3B_z)/(2\Delta B \gamma_{3D}) - 1}. \tag{S42}$$

This relationship implies that both the LD value and the anisotropy factor $r$ also suffer from bias; a molecule always exhibits an emission pattern of a more rotationally-fixed molecule for finite SNR.

### F. Multipole emitter analysis

In the main text, we model a fluorescent molecule as a radiating dipole $\boldsymbol{\mu}$. This approximation is accurate in far-field fluorescence imaging, e.g., STED [6], STORM [7] and (f)PALM [8, 9]. Since the higher multipole orders interact with the divergence of the electric field, they become negligible when the electric field is sufficiently homogeneous over the dimension of the particle for far-field excitation or when the emission is viewed in the far field [10]. In near-field optics, e.g., field-enhanced scanning near-field optical microscopy [11], the dipole approximation might be insufficient to model the interaction between nanoparticles and the electric field. Here, we briefly introduce the effect of the quadrupole using an excitation-based example.

The electric quadrupole is defined as [10]

$$\boldsymbol{Q} = [Q_{xx}, Q_{yy}, Q_{zz}, Q_{xy}, Q_{xz}, Q_{yz}]^\dagger. \tag{S43}$$

The emitted intensity $g_i$ in response to excitation by the electric field $\boldsymbol{E}_i$ is given by

$$g_i = s\left|\left(\left[\frac{\partial}{\partial x}, \frac{\partial}{\partial y}, \frac{\partial}{\partial z}, \frac{\partial}{\partial x} + \frac{\partial}{\partial y}, \frac{\partial}{\partial x} + \frac{\partial}{\partial z}, \frac{\partial}{\partial y} + \frac{\partial}{\partial z}\right](\mathbf{1}^\dagger \boldsymbol{E}_i)\right)\boldsymbol{Q}\right|^2 + b_i. \tag{S44}$$

Since the quadrupole vector $\boldsymbol{Q}$ has 5 degrees of freedom ($Q_{xx} + Q_{yy} + Q_{zz} = 0$), the rotational constraint $\gamma_{\boldsymbol{Q}}$ is defined differently from $\gamma_{\text{2D}}$ and $\gamma_{\text{3D}}$, which are derived from dipoles $\boldsymbol{\zeta}$ (1 degree of freedom) and $\boldsymbol{\mu}$ (2 degrees of freedom), respectively. However, this forward imaging model is similar to Eq. (S1), and the measured fluorescence is dependent upon the second-order moments of the quadrupole $\boldsymbol{Q}$. Therefore, our theoretical framework to analyze the bias in rotational constraint can be easily extended and applied to higher-order multipoles as well.

[1] A. S. Backer, M. Y. Lee, and W. E. Moerner, Optica **3**, 659 (2016).

[2] O. Zhang, J. Lu, T. Ding, and M. D. Lew, Applied Physics Letters **113**, 031103 (2018).

[3] K. I. Mortensen, L. S. Churchman, J. A. Spudich, and H. Flyvbjerg, Nature Methods **7**, 377 (2010).

[4] M. A. Lieb, J. M. Zavislan, and L. Novotny, Journal of the Optical Society of America B **21**, 1210 (2004).

[5] J. R. Lakowicz, *Principles of Fluorescence Spectroscopy* (Springer Science+Business Media, New York, 2006).

[6] S. W. Hell and J. Wichmann, Optics letters **19**, 780 (1994).

[7] M. J. Rust, M. Bates, and X. Zhuang, Nature Methods **3**, 793 (2006).

[8] E. Betzig, G. H. Patterson, R. Sougrat, O. W. Lindwasser, S. Olenych, J. S. Bonifacino, M. W. Davidson, J. Lippincott-Schwartz, and H. F. Hess, Science **313**, 1642 (2006).

[9] S. T. Hess, T. P. Girirajan, and M. D. Mason, Biophysical Journal **91**, 4258 (2006).

[10] L. Novotny and B. Hecht, *Principles of Nano-Optics* (Cambridge University Press, Cambridge, England, 2012).

[11] A. Bouhelier, Microscopy research and technique **69**, 563 (2006).

## III. SUPPLEMENTAL FIGURES

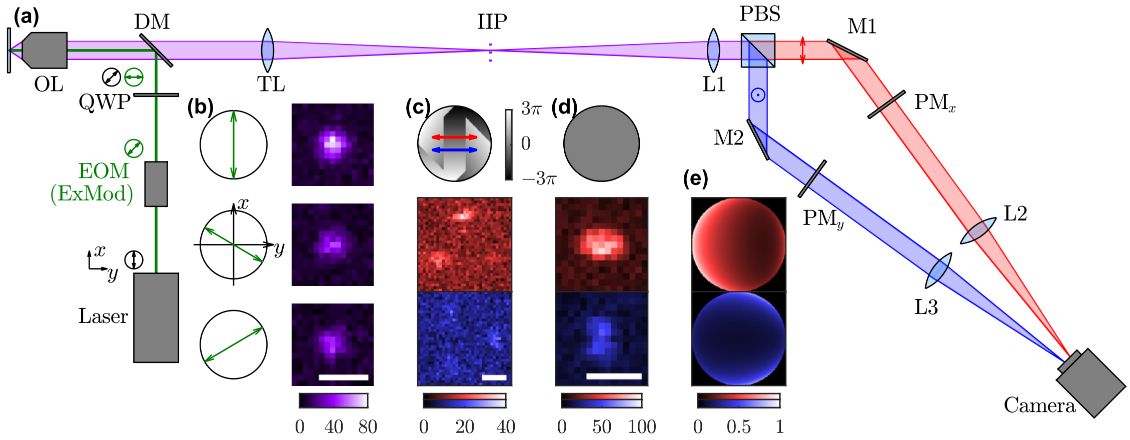


FIG. S1. Schematics of various orientation-sensing methods. (a) Example imaging system. An excitation laser is modulated by an electro-optic modulator (EOM, only for excitation modulation method) and a quarter-wave plate (QWP, green: fast-axis orientation for excitation modulation, black: fast-axis orientation for all other methods), and then guided to the sample by a dichroic mirror (DM). Fluorescence is collected by an objective lens (OL, simulation $NA = 1.4$). An image is formed by the tube lens (TL) at the intermediate image plane (IIP). For all methods except excitation modulation, the fluorescence is split by a polarizing beam splitter (PBS) into two orthogonally-polarized channels. A $4f$ system is used to project the back focal plane (BFP) onto the phase masks ($PM_x$ and $PM_y$) and the final image plane onto a camera. The phase mask applied to the $y$-polarized channel $PM_y$ is identical to that applied to the $x$-polarized channel ($PM_x$), rotated clockwise by 90°. (b) Concept of the in-plane excitation modulation method. Images of molecules excited by three polarizations (green arrows) are captured at IIP. (c) Concept of the Tri-spot PSF. The Tri-spot phase mask (colorbar: phase in rad) is applied to the BFP. Images in both polarization channels are captured by the camera. Red: $x$-channel; Blue: $y$-channel. (d) Concept of the standard PSF. A flat phase mask (clear aperture) is applied to the BFP. (e) Concept of BFP imaging. Images are taken at the back focal plane after separating $x$- and $y$-polarized light into two channels. Colorbar: (b-d): photons detected, (e): Normalized intensity. Scale bar: 500 nm.

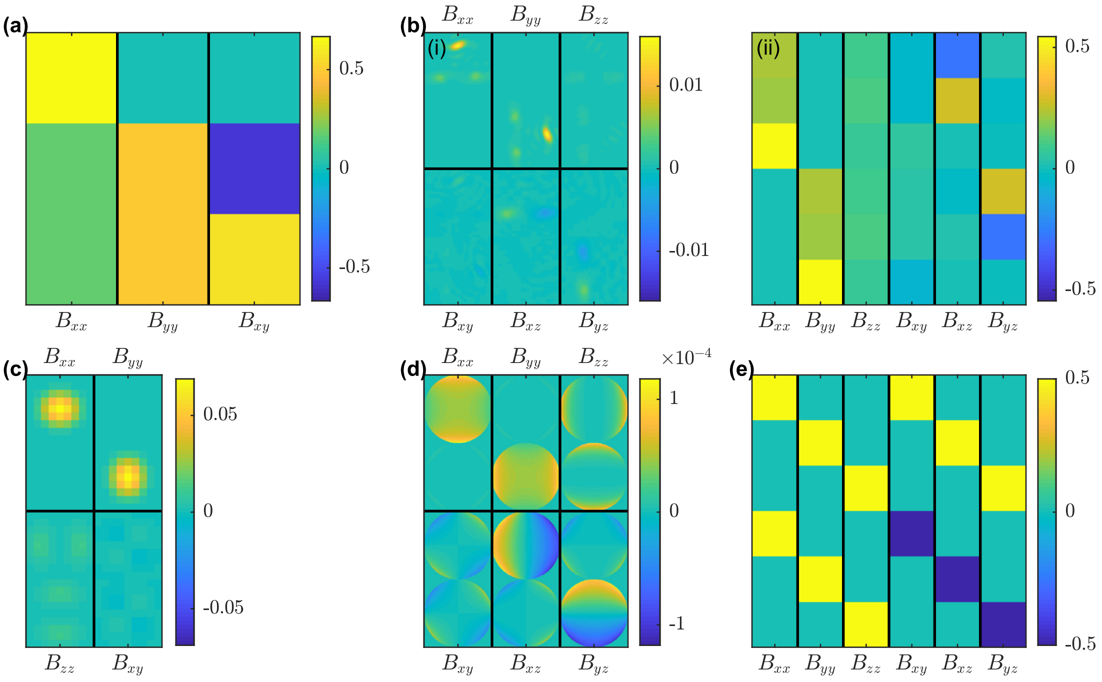


FIG. S2. (a) Second-moment matrix of excitation polarization modulation $\boldsymbol{B}_{\text{ExMod}}$. Each column of the 3-by-3 matrix represents one basis-image vector, while each row represents one integrated image $g_i$. (b)(i) Basis images of the Tri-spot PSF, which can be represented as (ii) a 6-by-6 basis-image matrix $\boldsymbol{B}_{\text{Tri-spot}}$ consisting of the relative brightness of the six diffraction-limited spots in each basis image. (c) Basis images of the standard PSF; each basis image is reshaped into a 162-vector, and then assembled into a 162-by-4 basis-image matrix $\boldsymbol{B}_{\text{standard}}$. (d) Basis images of the BFP; each basis image is reshaped into a 40212-vector ($\lfloor \pi 80^2 \rceil \times 2$, where $\lfloor \cdot \rceil$ denotes the rounding operator), and then assembled into a 40212-by-6 basis-image matrix $\boldsymbol{B}_{\text{BFP}}$. (e) Basis-image matrix of the ideal 3D measurement $\boldsymbol{B}_{\text{ideal}}$. Colorbar: normalized intensity.

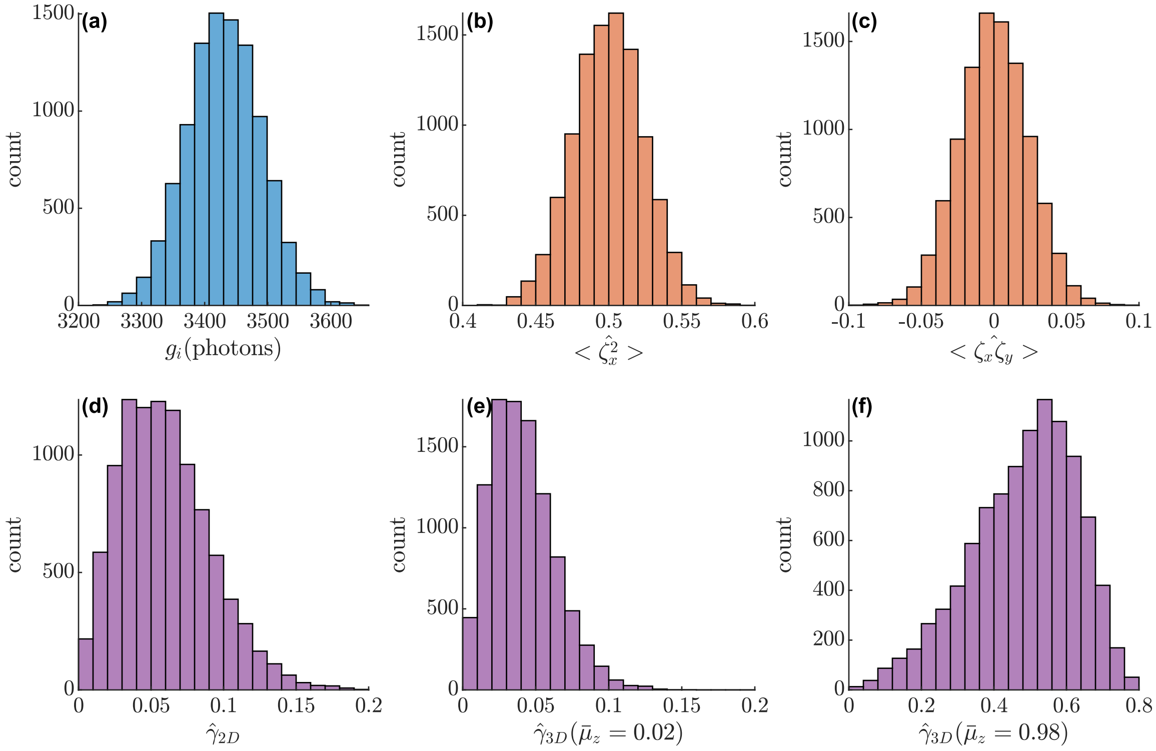


FIG. S3. Measuring the rotational constraint of an isotropic emitter using 10,000 simulated images for an SNR of $s = 3000$ and $\mathbf{1}^\dagger \boldsymbol{b} = 7290$ photons with Poisson noise using excitation modulation. (a) Distribution of the integrated photons $\boldsymbol{g}_i$ from one frame in a $526.5 \times 526.5$ nm$^2$ region of the camera. The measured orientational second moments (b) $\langle \hat{\zeta_x^2} \rangle$ and (c) $\langle \hat{\zeta_x \zeta_y} \rangle$ are both unbiased. (The bias in $\langle \bar{\hat{\zeta_x^2}} \rangle$ and $\langle \bar{\hat{\zeta_x \zeta_y}} \rangle$ are $3 \times 10^{-5}$ and $5 \times 10^{-5}$, respectively, both smaller than 1% of the estimation precision $\sigma_{\langle \hat{\zeta_x^2} \rangle} = \sigma_{\langle \hat{\zeta_x \zeta_y} \rangle} = 0.02$). (d) The distribution of rotational constraint (Eq. (3)) estimates $\hat{\gamma}_{\text{2D}}$ follows a non-central chi distribution (Eq. (4)), and the average $\bar{\hat{\gamma}}_{\text{2D}} = 0.06$ is consistent with Eq. (5). The computed 3D rotational constraints $\hat{\gamma}_{\text{3D}}$ based on Eq. (8) exhibit different distributions depending on the assumed out-of-plane orientation (e) $\bar{\mu}_z = 0.02$ versus (f) $\bar{\mu}_z = 0.98$.

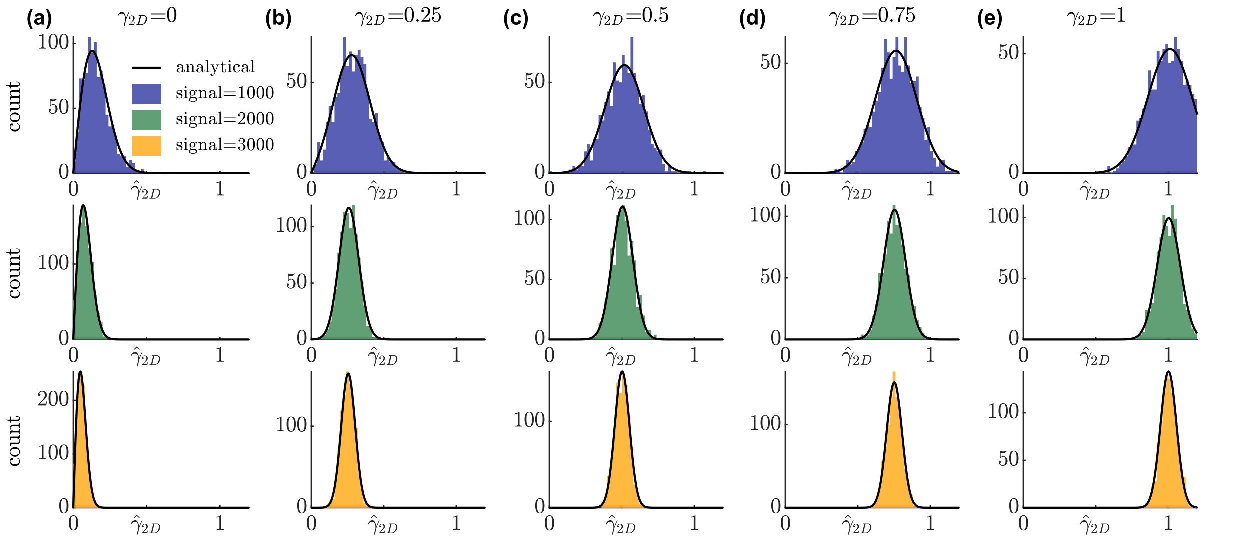


FIG. S4. Comparison between the analytical distribution of $\hat{\gamma}_{\mathrm{2D}}$ (solid lines, scaled non-central chi PDF given in Eq. (4)) and the measurements $\hat{\gamma}_{\mathrm{2D}}$ using a basis-inversion estimator (histograms, Section II A) on 1000 simulated images with in-plane excitation modulation. Images were simulated with molecular rotational constraints of (a) $\gamma_{\mathrm{2D}} = 0$, (b) $\gamma_{\mathrm{2D}} = 0.25$, (c) $\gamma_{\mathrm{2D}} = 0.5$, (d) $\gamma_{\mathrm{2D}} = 0.75$, and (e) $\gamma_{\mathrm{2D}} = 1$ and background photons of $\mathbf{1}^\dagger \boldsymbol{b} = 7290$ (30 per $58.5 \times 58.5\ \mathrm{nm}^2$ per frame). Blue, green, and yellow represent a signal level of 1000, 2000, and 3000 photons, respectively.

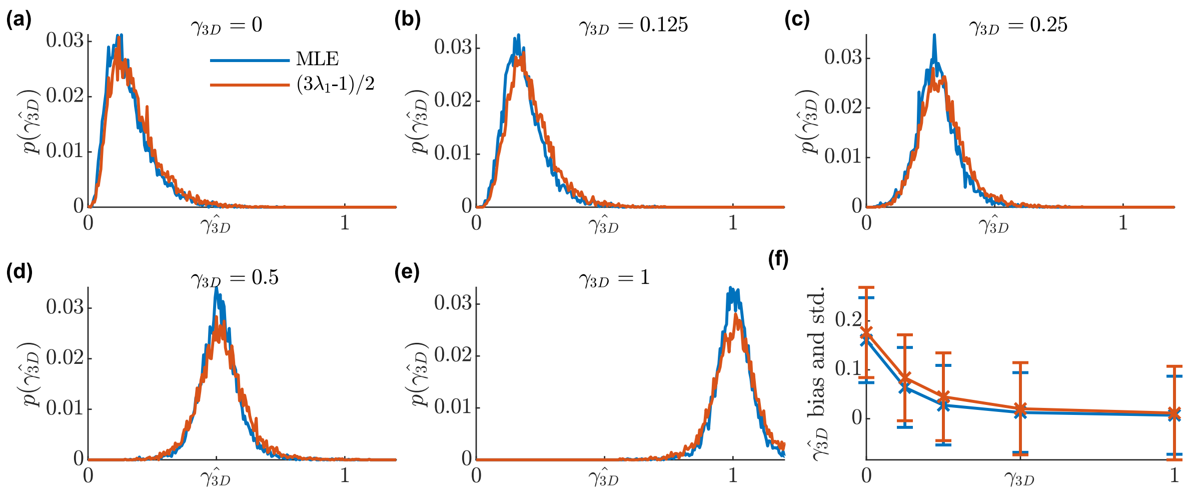


FIG. S5. Comparison between rotational constraint measurements using an eigendecomposition of the second-moment matrix (Eq. (S12)) versus a maximum-likelihood estimator (MLE, Eq. (S13)). The distribution of apparent rotational constraint $\hat{\gamma}_{3\text{D}}$ based on 9000 simulated images of the Tri-spot PSF for molecules with true rotational constraints of (a) $\gamma_{3\text{D}} = 0$, (b) $\gamma_{3\text{D}} = 0.125$, (c) $\gamma_{3\text{D}} = 0.25$, (d) $\gamma_{3\text{D}} = 0.5$, and (e) $\gamma_{3\text{D}} = 1$ and $s = 3000$ signal photons and $\mathbf{1}^\dagger \boldsymbol{b} = 4860$ background photons per spot (10 per $58.5 \times 58.5$ nm$^2$ in each polarization channel). Blue: MLE; red: eigendecomposition. (f) The bias and standard deviation are very similar for both estimators. Cross: bias; Errorbar: $\pm 1$ standard deviation.

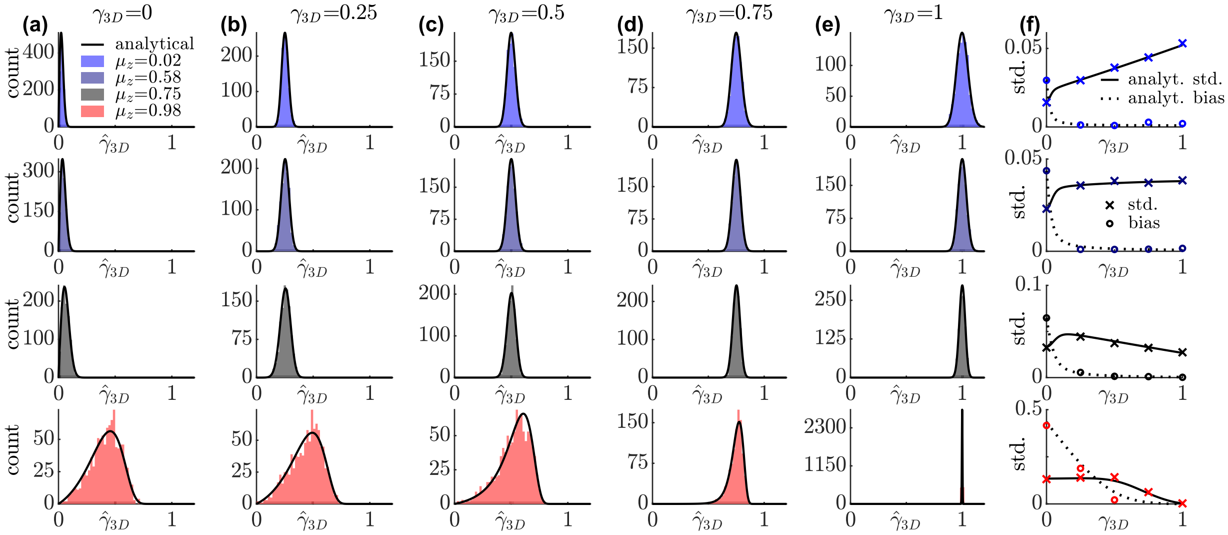


FIG. S6. Comparison between the analytical distribution of $\hat{\gamma}_{\mathrm{3D}}$ (solid lines, computed PDF in Eq. (S25)) and measurements of $\hat{\gamma}_{\mathrm{3D}}$ using a basis-inversion estimator (histograms, Section II C) on 1000 simulated images collected by the in-plane excitation modulation technique. Images were simulated with molecular rotational constraints of (a) $\gamma_{\mathrm{3D}} = 0$, (b) $\gamma_{\mathrm{3D}} = 0.25$, (c) $\gamma_{\mathrm{3D}} = 0.5$, (d) $\gamma_{\mathrm{3D}} = 0.75$, and (e) $\gamma_{\mathrm{3D}} = 1$ and $s = 3000$ signal photons and $\mathbf{1}^\dagger \boldsymbol{b} = 1620$ background photons (6.67 per $58.5 \times 58.5$ nm$^2$ per frame). Light blue, dark blue, black, and red represent the out-of-plane orientations $\bar{\mu}_z$ of 0.02, 0.58, 0.75, and 0.98, respectively. (f) Bias and standard deviation of $\hat{\gamma}_{\mathrm{3D}}$ using Eq. (S26,S27) versus basis-inversion estimator. Solid line: analytical standard deviation, dashed line: analytical bias, cross: estimator standard deviation, circle: estimator bias.

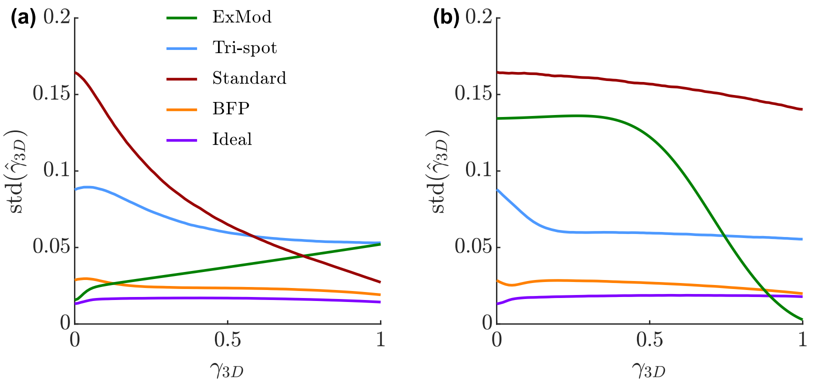


FIG. S7. Standard deviation of rotational constraint measurements of (a) horizontally- and (b) vertically-orientated fluorescent molecules using various techniques. Green: in-plane excitation modulation, blue: Tri-spot PSF, red: standard PSF, orange: back focal plane imaging, purple: ideal basis-image matrix. The extremely precise rotational constraint measurements using the excitation modulation method for highly-constrained, vertically-orientated molecules are due to the mapping between $\gamma_{\text{2D}}$ and $\gamma_{\text{3D}}$; measured 2D rotational constraints are mapped to a much narrower distribution in 3D.
